# Supplementary material for: Limitations of (Procrustes) Alignment in Assessing Multi-Person Human Pose and Shape Estimation
Source: arXiv:2409.16861 source file (2024-09-25)
Supplement: Supplementary file 1 [file 7_appendix.tex]

\section{Appendix}
\label{sec:annex}

\begin{figure}[!h]
    \centering
	    \includegraphics[width=0.86\columnwidth]{images/3_dataset_heatmap.png}
	\caption{Heat map of the action location per class (2D data).}
	\label{3data_heat}
\end{figure}

\begin{figure}[!h]
    \centering
	    \includegraphics[width=0.86\columnwidth]{images/3_dataset_hist.png}
	\caption{Histogram of the action location per class (3D data).}
	\label{3data_hist}
\end{figure}

\begin{figure}[!h]
\centering
    \begin{subfigure}{0.95\textwidth}
    \centering
        \includegraphics[width=\linewidth]{images/LSTM03D_loss_acc.png}
        \caption{\label{6app_loss_evoCS}Basic model.}
    \end{subfigure}
    \begin{subfigure}{0.95\textwidth}
    \centering
        \includegraphics[width=\linewidth]{images/LSTM03Dmasked_loss_acc.png}
        \caption{\label{6app_loss_evoMS}Masked model.}
    \end{subfigure}
    \begin{subfigure}{0.95\textwidth}
    \centering
        \includegraphics[width=\linewidth]{images/LSTM03Dpart_loss_acc.png}
        \caption{\label{6app_loss_evoTS}Trunc model.}
    \end{subfigure}
	\caption{\label{6app_loss_evo}Evolution of the loss for each of the models.}
\end{figure}

\begin{figure}[!h]
    \centering
	    \includegraphics[width=0.9\columnwidth]{images/acc_per_skeleton_percentage_val.png}
	\caption{Accuracy per percentage of skeleton available.}
	\label{6app_perMasked}
\end{figure}

\begin{figure}[!h]
    \centering
	    \includegraphics[width=0.9\columnwidth]{images/accuracy_per_percentage_val.png}
	\caption{Accuracy per percentage of the sequence available.}
	\label{6app_perTrunc}
\end{figure}

\begin{figure}[!h]
    \centering
	    \includegraphics[width=0.9\columnwidth]{images/accuracy_succesive_val_copy.png}
	\caption{Accuracy per actions (lines) given a previous one (columns).}
	\label{6app_consec3}
\end{figure}

\begin{figure}[!h]
    \centering
	    \includegraphics[width=0.9\columnwidth]{images/accuracy_succesive_bis_val_copy.png}
	\caption{Accuracy per actions (lines) given a previous one (columns) using a time window of 100 frames.}
	\label{6app_consec3win100}
\end{figure}

\begin{figure}[!h]
    \centering
	    \includegraphics[width=0.9\columnwidth]{images/accuracy_succesive_bis_val_3_copy.png}
	\caption{Accuracy per actions (lines) given a previous one (columns) using a time window of 75 frames.}
	\label{6app_consec3win175}
\end{figure}

\begin{figure}[!h]
\centering
    \begin{subfigure}{0.7\textwidth}
    \centering
        \includegraphics[width=\linewidth]{images/LSTM3DF_0.png}
        \caption{\label{6app_loss_evoCS}Basic model.}
    \end{subfigure}
    \begin{subfigure}{0.7\textwidth}
    \centering
        \includegraphics[width=\linewidth]{images/LSTM3DF_1.png}
        \caption{\label{6app_loss_evoMS}Masked model.}
    \end{subfigure}
	\caption{\label{6app_loss_evoF}Evolution of the loss for each of the final models.}
\end{figure}

\begin{figure}[!h]
    \centering
	    \includegraphics[width=0.9\columnwidth]{images/acc_per_skeleton_percentage_trainF_01.png}
	\caption{Accuracy per percentage of skeleton available..}
	\label{6app_perMF}
\end{figure}

\begin{figure}[!h]
    \centering
	    \includegraphics[width=0.9\columnwidth]{images/accuracy_per_percentage_trainF_01.png}
	\caption{Accuracy per percentage of the sequence available.}
	\label{6app_perSF}
\end{figure}

\begin{figure}[!h]
    \centering
	    \includegraphics[width=\columnwidth]{images/accuracy_succesive_trainF_01.png}
	\caption{Accuracy per actions (lines) given a previous one (columns).}
	\label{6app_consec2}
\end{figure}

\begin{figure}[!h]
\centering
    \begin{subfigure}{0.35\columnwidth}
    \centering
	    \includegraphics[width=\linewidth]{images/accuracy_succesive_bis_train_3FA.png}
	    \caption{Accuracy.}
    \end{subfigure}
    \hspace{2 cm}
    \begin{subfigure}{0.35\columnwidth}
    \centering
	    \includegraphics[width=\linewidth]{images/accuracy_succesive_bis_train_3FB.png}
	    \caption{Average number of frames to switch.}
    \end{subfigure}
    \caption{Accuracy per actions (lines) given a previous one (columns) using a time window of 100 frames.}
	\label{6app_consec2win100}
\end{figure}
